# Supplementary material for: Typical case behaviour of spin systems in random graph and composite ensembles
Source: arXiv:0904.2506 source file (2009-05-22)
Supplement: Supplementary file 1 [file Acronyms.tex]

%%Acronyms
